# Supplementary material for: Model-Twin Randomization (MoTR) for Estimating the Recurring Individual Treatment Effect
Source: arXiv:2208.00739 source file (2025-09-27)
Supplement: Supplementary file 1 [file appendix.tex]

\documentclass{article}
\usepackage[paperwidth=8.5in, paperheight=11in, margin=1in]{geometry}

\usepackage{array} % for extrarowheight
\usepackage{comment} % to use \begin{comment} and \end{comment}
\usepackage{afterpage}

% Figure symbols.
% http://texdoc.net/texmf-dist/doc/latex/wasysym/wasysym.pdf
% http://www.tex.ac.uk/tex-archive/info/symbols/comprehensive/symbols-a4.pdf
% http://tex.stackexchange.com/questions/100424/how-to-use-the-ifsym-package
\usepackage{wasysym}
\usepackage[geometry]{ifsym}

\usepackage{bm}

\usepackage{amssymb, amsmath, amsfonts, latexsym}
\usepackage[mathscr]{euscript}

% To add ceiling and floor brackets.
\usepackage{mathtools}

% To add equation and other fancy reference labels.
\usepackage{fancyref}

\usepackage{rotating}

\usepackage{multirow}
\usepackage{array, makecell, rotating}

% Math Symbol: Independence: User Definition

% Here's a version from http://jblevins.org/notes/latex#independence

% diamond with plus; taken from http://tex.stackexchange.com/questions/44073/overstruck-diamond-and-plus-in-plain-tex
\font\Bigmath=cmsy10 scaled \magstep2

\def\diamondplustwo{\mathrel{%
  \ooalign{$+$\cr\hss\lower.255ex\hbox{\Bigmath\char5}\hss}}}% multicolumn and multirow package

% Define control sequences.

 % coefficient of variation
 % empirical standard deviation

% Causal diagrams: Directed Acyclic Graphs. DAG-drawing package. http://www.konstantinkashin.com/blog/2013/06/19/dags-in-latex/
%\usepackage{pgf,tikz}
\usepackage{tikz}
\usetikzlibrary{arrows,decorations.pathmorphing,backgrounds,positioning,fit,petri}

\usepackage{tabu} % to use extrarowsep

\usepackage[square]{natbib}

\usepackage{fancyhdr}
\pagestyle{fancy}
\lhead{{\footnotesize Appendix for \lq\lq Model-Twin Randomization (MoTR) for Estimating One's Own Average Individual Treatment Effect \hdots"}}
\rhead{{Daza, Eric J.}}
\lfoot{PRE-PRINT ONLY as of \today}
\rfoot{CONFIDENTIAL: DO NOT DISTRIBUTE}

% Add line numbers for easy referencing for revisions.
% WARNING: MAKE SURE TO ADD SPACE BEFORE EACH ALIGN ARGUMENT, OR ELSE THE PRECEDING PARAGRAPH LINES WILL NOT BE NUMBERED!!!! http://tex.stackexchange.com/questions/43648/why-doesnt-lineno-number-a-paragraph-when-it-is-followed-by-an-align-equation
% \usepackage{lineno}
\usepackage[pagewise]{lineno} % to restart number per page
\linenumbers

% Change spacing.
%\linespread{2.0}

% Remove brackets from Reference numbering (i.e., [1] --> 1.).
\makeatletter \renewcommand\@biblabel[1]{#1.} \makeatother

% Use these to refer to labels in rubin.granger_main.tex.
%\usepackage{xr}
%\externaldocument{rubin.granger_main}
\usepackage{zref-xr}
\zxrsetup{tozreflabel=false, toltxlabel=true, verbose}
\zexternaldocument*{rubin.granger_main}

% % Include watermark.
% \usepackage{draftwatermark}
% %\SetWatermarkText{Do Not Distribute}
% % \SetWatermarkText{\textsc{Do Not Distribute}}
% \SetWatermarkScale{2.5}
% \SetWatermarkColor[gray]{0.91}

\begin{document}

\input appendix/appendix_body

\bibliographystyle{vancouver}
\bibliography{references}

\end{document}
